# Supplementary material for: Entity Anchored ICD Coding
Source: arXiv:2208.07444 source file (2022-08-15)
Supplement: Supplementary file 1 [file appendix.tex]

% \appendix

% \section{Hyperparameter Search}
